# Supplementary material for: Fast, accurate, and system-specific variable-resolution modelling of proteins
Source: arXiv:2207.03187 ancillary file (2023-01-19)
Supplement: Supplementary file 1 [file SI.pdf]

# Supporting Information for: Fast, accurate, and system-specific variable-resolution modelling of proteins

Raffaele Fiorentini<sup>1,2</sup>, Thomas Tarenzi<sup>1,2</sup>, Raffaello Potestio<sup>1,2</sup>

<sup>1</sup>*Physics Department, University of Trento, Via Sommarive 14, Povo (TN), Italy*

<sup>2</sup>*INFN-TIFPA, Trento Institute for Fundamental Physics and Applications, Via Sommarive 14, Povo (TN), Italy*

## S1 Derivation of the elastic constants $k_{nb}$

As discussed in the main text, in the CANVAS model two non-consecutive  $C_\alpha$  beads—be they part of “medium” or “coarse grained” residues as prescribed by the CANVAS scheme—are connected *via* a harmonic potential of stiffness  $k_{nb}$  if their distance in the reference (native) conformation of the system lies within a cutoff of 1.4 nm. Importantly, the magnitude of  $k_{nb}$  decreases as the distance  $d$  between the pair of  $C_\alpha$ ’s increases; in this section, we will describe all the technical details involved in the parameterisation of  $k_{nb}(d)$ .

Firstly, we extracted from the all-atom MD simulations of pembrolizumab [1] a subset of the probability distributions  $P_{ij}(r_{ij})$  of the scalar distance  $r_{ij} = |\mathbf{r}_i - \mathbf{r}_j|$  between two non-consecutive  $\alpha$ -carbon atoms  $C_{\alpha,i}$  and  $C_{\alpha,j}$ , where  $i, j = 1, \dots, N_R$  run over the  $N_R$  total residues in the system. This analysis was conducted separately for each chain composing the macromolecule, and further restricting the set of possible  $C_{\alpha,i}$ — $C_{\alpha,j}$  pairs to all those whose separation along the sequence satisfies  $1 < j - i < 16$ —thus neglecting consecutive residues. Starting from the set of  $P_{ij}(r_{ij})$ , we then relied on the direct Boltzmann inversion method [2] to determine an effective, harmonic pair potential  $V_{ij}(r) = \frac{1}{2}k_{ij}(r_{ij} - r_{ij}^0)^2$  acting among each pair of  $C_\alpha$  sites. The associated harmonic constants  $k_{ij}$ —actually, the combination  $\beta k_{ij}$ , with  $\beta = 1/k_B T$ —and equilibrium distances  $r_{ij}^0$  were obtained by separately fitting each  $P_{ij}(r_{ij})/r_{ij}^2$  to a Gaussian distribution.

Distal residues along the sequence are not necessarily distant in the three dimensional conformation of the system. As such, the resulting ensemble of harmonic constants  $\beta k_{ij}$  was then binned according to the spatial distance  $d$  between the associated  $\alpha$ -carbon atoms in the reference (native) conformation of the antibody. The distance-dependent spring constant  $\beta k_{nb}(d_n)$  at distance  $d_n$  was then determined as the average

of all the  $\beta k_{ij}$  contained in bin  $[d_n, d_n + \Delta]$ , with  $\Delta = 0.1$  nm and on an overall interval  $[d_{min}, d_{max}] = [0.4, 4.5]$  nm.

The results obtained for  $\beta k_{nb}(d)$  are presented in Figure S1. We note that  $\beta k_{nb}(d)$  displays a steep decrease for short separations, gradually moving towards a plateau for increasing distance between the two  $C_\alpha$  beads. Importantly, although we determined  $\beta k_{nb}(d)$  up to  $d_{max} = 4.5$  nm, we again stress that in the CANVAS model two  $C_\alpha$  beads are connected by a weak spring only if their distance in the native conformation is smaller than 1.4 nm. Finally, to avoid, in the force field parameters of CANVAS, the presence of abrupt changes in the weak spring constant  $k_{nb}$  for slight variations of the distance, the data for  $\beta k_{nb}(d)$  were fit to a power law  $f(d) = \gamma + \delta d^\alpha$ , finding  $\gamma = 81.22$  nm<sup>-2</sup>,  $\delta = 1322.06$  nm<sup>-2</sup>, and  $\alpha = -1.26$ . Results for the fit are included in Figure S1, and display that the fitting function captures the overall behavior of the raw  $\beta k_{nb}(d)$  data points within the region relevant for CANVAS, that is, for  $d \in [0.4, 1.4]$  nm.

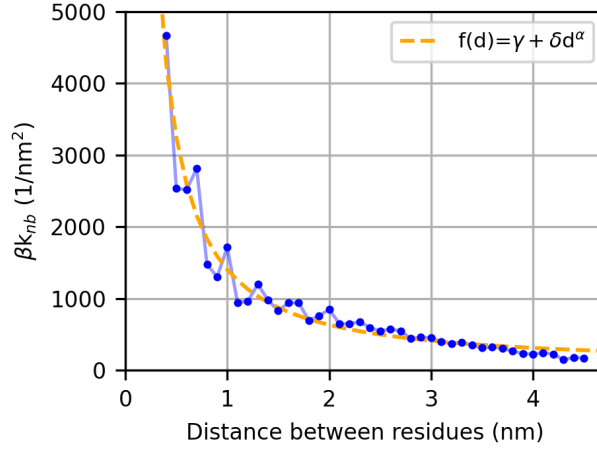

Figure S1: Dependence of the harmonic constants with respect to the spatial distance between  $C_\alpha$  atoms. Data are fitted with the orange dashed curve, as described in the text.

## S2 Supplementary figures

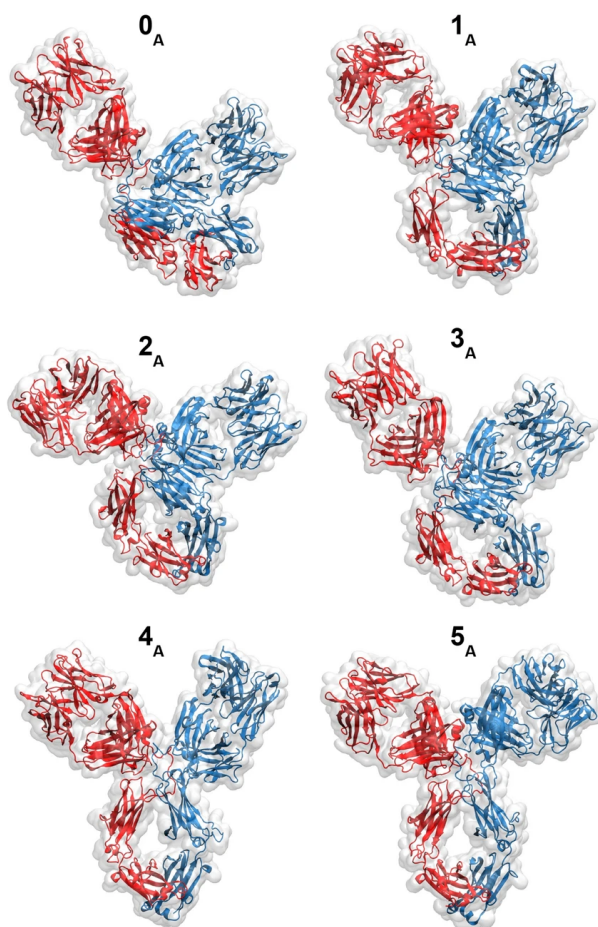

Figure S2: Representative structures of deglycosylated pembrolizumab in the apo form, for each conformational cluster. Chains A and B are in blue, and chains C and D in red. Figure adapted from Ref. [1].

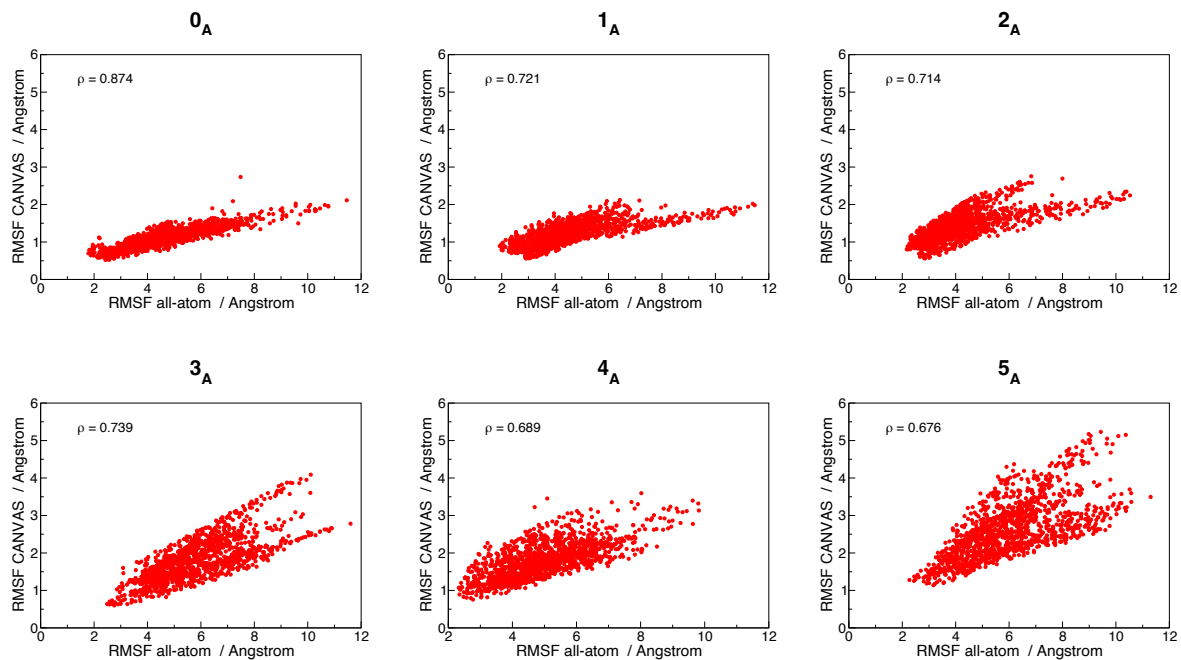

Figure S3: Scatter plots of RMSF for each apo form of pembrolizumab, comparing the results of all-atom simulation and CANVAS one.  $\rho$  indicates the value of Pearson Coefficient computed between the two sets of fluctuations. All clusters show satisfactory results: an excellent correlation is found in 0<sub>A</sub> cluster ( $\rho \sim 0.87$ ); the other clusters present good RMSF correlations ( $\rho \sim 0.7$ ).

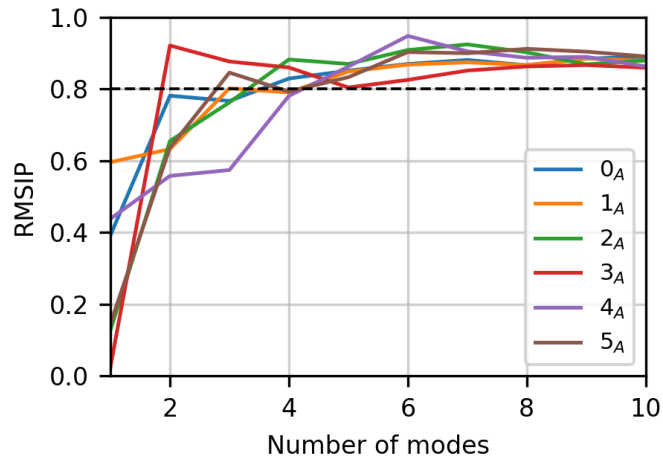

Figure S4: RMSIP between the essential subspaces computed from the atomistic and CANVAS simulations. In all clusters, 5 modes (or even less) are sufficient to reach an RMSIP larger than 0.8, indicating a very good overlap [3].

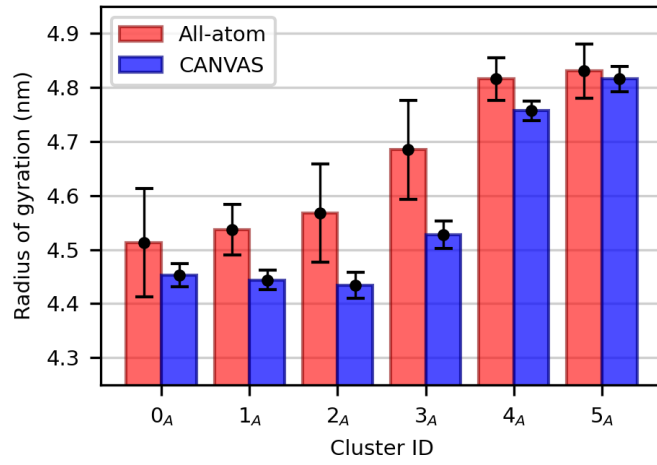

Figure S5: Average radius of gyration computed for each conformational cluster of the antibody, in the all-atom and multiscale representations. In both cases, only the positions of  $C_{\alpha}$  atoms and CA beads were taken into account. Results from the all-atom case are taken from Ref. [1].

## References

- [1] T. Tarenzi, M. Rigoli, and R. Potestio, “Communication pathways bridge local and global conformations in an igg4 antibody,” *Scientific reports*, vol. 11, no. 1, pp. 1–12, 2021.
- [2] D. Reith, M. Pütz, and F. Müller-Plathe, “Deriving effective mesoscale potentials from atomistic simulations,” *Journal of computational chemistry*, vol. 24, no. 13, pp. 1624–1636, 2003.
- [3] A. Amadei, M. A. Ceruso, and A. Di Nola, “On the convergence of the conformational coordinates basis set obtained by the essential dynamics analysis of proteins’ molecular dynamics simulations,” *Proteins: Structure, Function, and Bioinformatics*, vol. 36, no. 4, pp. 419–424, 1999.
